# Supplementary material for: Fair Robust Active Learning by Joint Inconsistency
Source: arXiv:2209.10729 source file (2022-11-17)
Supplement: Supplementary file 1 [file supp.pdf]

# Supplementary Material for “Fair Robust Active Learning by Joint Inconsistency”

Tsung-Han Wu<sup>1</sup>, Shang-Tse Chen<sup>1</sup>, and Winston H. Hsu<sup>1,2</sup>

<sup>1</sup> National Taiwan University    <sup>2</sup> Mobile Drive Technology

## Implementation Details

We introduce our computing infrastructure, dataset preprocessing, and training details in this section.

### Computing Infrastructure

All experiments are conducted on an 8-core CPU personal computer with an NVIDIA RTX3090 GPU. Besides, the computational comparison shown in Tab. 2 in the main paper is evaluated on this machine.

### Dataset Preprocessing

**UTKFace.** We conducted the four race (White, Black, Asian, and Indian) classification problem (Karkkainen et al. 2021) and utilize age as the sensitive attribute on this dataset. In our preprocessing pipeline, we first filter out face photos belonging to the “Other” race. Then, we put an age-related attribute tag on each photo based on the provided age metadata. Specifically, we nearly evenly partition all faces into two groups, Young and Old, with the threshold of 30 years old. Finally, we split the data into training and testing sets with a ratio of 7 : 3. We train the network with resized images,  $112 \times 112$ , for speed consideration.

**CINIC-10.** We conducted the official ten objects classification problem (Darlow et al. 2018) and utilize the membership in a particular domain (CIFAR-10 or ImageNet) as the sensitive attribute on this dataset. The training and testing set in our experiments are identical to the official split. We train the network with the original image size,  $32 \times 32$ .

**HAM-10000.** We conducted the official seven cell type classification problem (Tschandl et al. 2018) and utilize genders as sensitive attributes on this dataset. In our preprocessing pipeline, we first filter out duplicated images and samples without a corresponding sex attribute. Then, we split the data into training and testing sets with a ratio of 7 : 3. We train the network with resized images,  $112 \times 112$ , for speed consideration.

**Initial Labeled Data in Active Learning.** We randomly and uniformly select 20% of the data in the training set as the initial labeled set, and treat the other 80% as the unlabeled data pool. We have confirmed that the data distribution of the partitioned two subsets are similar to the original distribution.

## Training Details

The overall framework of our proposed Joint INconsistency method (JIN) is provided in Algo. 1 in the main paper. Here we focus on the more detailed model training process, including the implementation of attack and defense methods as well as a conventional deep neural network pipeline.

**Adversarial Attack and Defense.** We utilize the python foolbox package (Rauber, Brendel, and Bethge 2017) to achieve the PGD adversarial attacks in all our experiments. Likewise, in all experiments, we implement the TRADES adversarial training (Zhang et al. 2019) while directly leveraging the official GitHub repository<sup>1</sup>.

**Deep Neural Network Pipeline.** In the following, we elaborate on our deep neural network adversarial training and fine-tuning pipeline (corresponding to the “Adv-Train” in Algo. 1 of the main paper). For three datasets, we leverage the SGD optimizer to train our model with an initial learning rate of  $\gamma$ , a momentum of  $\mu$ , and a weight decay  $\lambda$ . For each active learning iteration, we adversarially train the model for  $E$  epochs with a batch size of  $B$ . To make the whole training pipeline stable, we utilize the cosine annealing learning rate scheduler with a warm-up stage of initial  $E_w$  epochs.

For the UTKFace dataset, we set  $\gamma = 0.1$ ,  $\mu = 0.9$ ,  $\lambda = 2e-4$ ,  $E = 70$ ,  $E_w = 10$ , and  $B = 32$ . For the CINIC-10 dataset, we set  $\gamma = 0.1$ ,  $\mu = 0.9$ ,  $\lambda = 2e-4$ ,  $E = 100$ ,  $E_w = 10$  and  $B = 64$ . For the HAM-10000 dataset, we set  $\gamma = 0.02$ ,  $\mu = 0.9$ ,  $\lambda = 2e-4$ ,  $E = 50$ ,  $E_w = 5$  and  $B = 32$ . Note that for a fair comparison, all models used in our experiments are not pre-trained.

## More Discussions

In the main text, we compare the performance of our proposed joint inconsistency method (JIN) with active learning and the FAL baselines. However, unlike traditional active learning approaches sampling from the whole unlabeled set, our method first estimate the worst group and select data from it to boost fairness metrics. Therefore, to ensure a fair comparison, we conduct further experiments on the UTK-Face dataset to compare our JIN method with the best active

<sup>1</sup><https://github.com/yaodongyu/TRADES>

learning approach (ENT) with only sampling data from the worst group, called G-ENT. The result is shown in Tab. 1.

|            | STD. Acc. (%)                    |                                  | Rob. Acc. (%)                    |                                  |
|------------|----------------------------------|----------------------------------|----------------------------------|----------------------------------|
|            | Worst ( $\uparrow$ )             | Avg. ( $\uparrow$ )              | Worst ( $\uparrow$ )             | Avg. ( $\uparrow$ )              |
| ENT        | 74.10 $\pm$ 0.79                 | 75.33 $\pm$ 0.56                 | 56.94 $\pm$ 0.64                 | <b>60.25<math>\pm</math>0.56</b> |
| G-ENT      | 68.14 $\pm$ 0.62                 | 70.56 $\pm$ 0.44                 | 54.89 $\pm$ 0.32                 | 58.85 $\pm$ 0.37                 |
| <b>JIN</b> | <b>75.07<math>\pm</math>0.53</b> | <b>75.74<math>\pm</math>0.49</b> | <b>57.39<math>\pm</math>0.10</b> | 60.10 $\pm$ 0.25                 |

Table 1: More comparison on the UTKFace dataset.

The result shows that G-ENT even performs worse than the original ENT, including the worst group performance as well as the average performance. We gauge that the phenomenon may be due to sampling bias. Overall, in the experimental setting where only the worst group data are selected, our method still outperforms the best active learning method (ENT), demonstrating the effectiveness of our JIN method.

## References

- Darlow, L. N.; Crowley, E. J.; Antoniou, A.; Storkey, A. J.; et al. 2018. Cinic-10 is not imagenet or cifar-10. *arXiv preprint arXiv:1810.03505*.
- Karkkainen, K.; Joo, J.; others; et al. 2021. FairFace: Face Attribute Dataset for Balanced Race, Gender, and Age for Bias Measurement and Mitigation. In *Proceedings of the IEEE/CVF Winter Conference on Applications of Computer Vision*, 1548–1558.
- Rauber, J.; Brendel, W.; and Bethge, M. 2017. Foolbox: A Python toolbox to benchmark the robustness of machine learning models. In *Reliable Machine Learning in the Wild Workshop, 34th International Conference on Machine Learning*.
- Tschandl, P.; Rosendahl, C.; Kittler, H.; et al. 2018. The HAM10000 dataset, a large collection of multi-source dermatoscopic images of common pigmented skin lesions. *Scientific data*, 5(1): 1–9.
- Zhang, H.; Yu, Y.; Jiao, J.; Xing, E.; Ghaoui, L. E.; and Jordan, M. 2019. Theoretically Principled Trade-off between Robustness and Accuracy. In Chaudhuri, K.; and Salakhutdinov, R., eds., *Proceedings of the 36th International Conference on Machine Learning*, volume 97 of *Proceedings of Machine Learning Research*, 7472–7482. PMLR.
